# Supplementary material for: Federated Continual Learning with Weighted Inter-client Transfer
Source: arXiv:2003.03196 source file (2021-06-14)
Supplement: Supplementary file 1 [file 9_z3_n_clients.tex]

\subsection{Federated Continual Learning with Larger Number of Clients}
\label{sup:subsec:n_clients}
We further provide additional experimental results, including FedProx-APD, for the experiments with $5$, $20$, and $100$ clients over Overlapped-CIFAR-100 dataset. As shown in \Cref{sup:fig:fcl-cleint-perf} and \Cref{sub:tab:n_clients}, our FedWeIT consistently outperforms all baseline models for all experiments with $5$, $20$, and $100$ clients.

\begin{table}[t]
\caption{\small Average Per-task Performance on Overlapped-CIFAR-100 during FCL with $5$, $20$, and $100$ clients.}
\footnotesize
\centering
\begin{tabular}{l||c|c||c|c||c|c}
\hline
\hline
\multicolumn{1}{c||}{} & 
\multicolumn{2}{c||}{\textbf{5 clients}} &
\multicolumn{2}{c||}{\textbf{20 clients}} &
\multicolumn{2}{c}{\textbf{100 clients}}\\
\hline
\hline
\textbf{Methods} & 
\textbf{Accuracy ($\%$)} & \textbf{Capacity} & 
\textbf{Accuracy ($\%$)} & \textbf{Capacity} & 
\textbf{Accuracy ($\%$)} & \textbf{Capacity} \\
%\multicolumn{1}{c||}{\textbf{Methods}} & \multicolumn{4}{c}{\textbf{Fed-APC}}\\
\hline
\textbf{Local-STL} &
%\begin{tabular}{@{}c@{}} \textbf{54.70} \\ \textbf{$\pm$ 0.24}\end{tabular} &

57.15 \tiny{\tiny{$\pm$ 0.07}}&
1,000 \% &
39.66 \tiny{\tiny{$\pm$ 0.04}} &
1,000 \% &
32.96 \tiny{\tiny{$\pm$ 0.05}} &
1,000 \% \\
\textbf{Local-EWC} &
%\begin{tabular}{@{}c@{}} \textbf{54.70} \\ \textbf{$\pm$ 0.24}\end{tabular} &
44.26 \tiny{\tiny{$\pm$ 0.43}} &
100 \% &
41.30 \tiny{\tiny{$\pm$ 0.27}} &
100 \% &
25.33 \tiny{\tiny{$\pm$ 0.20}}&
100 \% \\
\textbf{Local-APD} &
%\begin{tabular}{@{}c@{}} \textbf{54.70} \\ \textbf{$\pm$ 0.24}\end{tabular} &
50.82 \tiny{\tiny{$\pm$ 0.33}} &
124 \% &
46.48 \tiny{\tiny{$\pm$ 0.26}} &
153 \% &
37.50 \tiny{\tiny{$\pm$ 0.22}} &
329 \% \\
\hdashline
\textbf{FedCurv} &
%\begin{tabular}{@{}c@{}} \textbf{54.70} \\ \textbf{$\pm$ 0.24}\end{tabular} &
40.36 \tiny{\tiny{$\pm$ 0.44}} &
100 \% &
33.05 \tiny{\tiny{$\pm$ 0.25}}&
100 \% &
29.11 \tiny{\tiny{$\pm$ 0.29}}&
100 \% \\
\textbf{~~~(+) EWC} &
%\begin{tabular}{@{}c@{}} \textbf{54.70} \\ \textbf{$\pm$ 0.24}\end{tabular} &
40.59 \tiny{\tiny{$\pm$ 0.31}} &
100 \% &
33.29 \tiny{\tiny{$\pm$ 0.37}}&
100 \% &
29.72 \tiny{\tiny{$\pm$ 0.20}}&
100 \% \\
%\textbf{FedProx-EWC} &
%\begin{tabular}{@{}c@{}} \textbf{54.70} \\ \textbf{$\pm$ 0.24}\end{tabular} &
%41.91\% &
%100\% &
%36.58\% &
%100\% &
%xx.xx\% &
%100\% \\
\textbf{FedProx-APD} &
%\begin{tabular}{@{}c@{}} \textbf{54.70} \\ \textbf{$\pm$ 0.24}\end{tabular} &
52.20 \tiny{\tiny{$\pm$ 0.31}}&
100 \% &
45.57 \tiny{\tiny{$\pm$ 0.27}}&
155 \% &
38.11 \tiny{\tiny{$\pm$ 0.27}}&
319 \% \\
\hdashline
\textbf{FedWeIT} &
\textbf{55.16} \tiny{\tiny{$\pm$ 0.19}} &
126 \% &
\textbf{50.38} \tiny{\tiny{$\pm$ 0.16}}&
155 \% &
\textbf{39.58} \tiny{\tiny{$\pm$ 0.17}}&
330 \% \\
\hline
\end{tabular}
\label{sub:tab:n_clients}
\end{table}
