# Supplementary material for: Federated Continual Learning with Weighted Inter-client Transfer
Source: arXiv:2003.03196 source file (2021-06-14)
Supplement: Supplementary file 3 [file 9_supplementary.tex]

\newpage
\appendix
\section{Appendix}

\input{supp/9_z1_sup_setting}
\input{supp/9_Z2_sup_data}
\input{supp/9_Z4_n_rounds}
\input{supp/9_z5_n_clients_plot}
\input{supp/9_z8_full_forgetting}
