# Supplementary material for: Federated Continual Learning with Weighted Inter-client Transfer
Source: arXiv:2003.03196 source file (2021-06-14)
Supplement: Supplementary file 7 [file 9_zz1_asyn_table.tex]

\begin{wraptable}{rb!}{1.8in}
\pu{\footnotesize
\vspace{-0.34in}
\caption{\footnotesize \pu{Averaged performance of FedWeIT with synchronous and asynchronous federated continual learning scenario.}}
\vspace{.05in}
\label{table:asyn}
\begin{tabular}{lc} 
\hline
\multicolumn{2}{c}{\textbf{NonIID-50}} \\ \hline \hline
\multicolumn{1}{c||}{\textbf{FedWeIT}} & \multicolumn{1}{c}{\textbf{Accuracy (\%)}}\\ \hline
\multicolumn{1}{l||}{\textbf{Synchronous}} & \multicolumn{1}{c}{\textbf{84.11 $\pm$ 0.27}} \\
\multicolumn{1}{l||}{\highlight{\textbf{Asynchronous}}} & \multicolumn{1}{c}{\textbf{84.40 $\pm$ 0.41}} \\
\hline
\end{tabular}
\vspace{-0.16in}
}\end{wraptable}
%\vspace{-0.1in}
